# Supplementary material for: Constrained Decoding of Diffusion LLMs with Context-Free Grammars
Source: arXiv:2508.10111 source file (2026-11-26)
Supplement: Supplementary file 2 [file app_case_study.tex]

\begin{table}[p]
    \caption{Three examples demonstrating the impact of constrained decoding on \dlm{} and \mri{} completion. Left are unconstrained completions (\vanilla{}) with problematic tokens highlighted in \wrongtok{red}, and right constrained completions (\constrained{}) with corrections highlighted in \righttok{green}, adapted for clarity. In (a) \dream{} our method corrects the type of values in a summary of a financial review for task \#30 in our \json{} dataset. In (b) \dreamcoder{} our method prevents closing more parentheses than are opened when generating a \smiles{} molecule for task \#166. In (c), \deepseekcsevenb{} our method forces adding parenthesis around a Python-style parentheses-less condition in an if-statement when writing a string processing function in task \#150 of our \humaneval{} dataset.}
  \label{fig:case-study}
  \vspace{2mm}
  \lstset{
  basicstyle=\small,
  breaklines=true,
  %frame = single,
  %frameround=tttt,
  %rulecolor=\color{black},
  %backgroundcolor = \color{lightgray},
  numbers=none,
  escapechar=\%,
  basicstyle=\linespread{0.7}\ttfamily\footnotesize,
  framexleftmargin=3mm, % Adjust left margin
  framexrightmargin=10mm,
  aboveskip=10mm,
  belowskip=10mm,
  }
  
  \small
  \centering
  \setlength{\tabcolsep}{8pt}
    \begin{tabular}{@{}l|l|l@{}}%{0.45\textwidth}|c{0.5\textwidth}}
        &\multicolumn{1}{c|}{\small Vanilla }&\multicolumn{1}{c}{\small Constrained}

        \\\hline
        {(a)}&
    \begin{lstlisting}[language=json]
// summarize my financial review

{
  "capitalGains": %\wrongtok{"5210.5000"}%,
  "interestIncome": %\wrongtok{"1340.25"}%,
  "totalReturn": %\wrongtok{"4.5"}%
}
%\hspace{1pt}%
    \end{lstlisting} &
    \begin{lstlisting}[language=json]
// summarize my financial review

{
  "capitalGains": %\righttok{5210.5000}%,
  "interestIncome": %\righttok{1340.25}%,
  "totalReturn": %\righttok{4.5}%
}
%\hspace{1pt}%
    \end{lstlisting}
        \hspace{1pt}
        \\
        \hline
        {(b)}&
    \begin{lstlisting}
// generate an allene with axial chirality

C1=CC1=CC(C(OO)O)C(OO)O%\wrongtok{)C(OO)O}%

    \end{lstlisting} &
    \begin{lstlisting}
// generate an allene with axial chirality

C1=CC1=CC(C(OO)O)C(OO)O
    \end{lstlisting}
        \hspace{1pt}
        \\[8mm]\hline
        {(c)}&
    \begin{lstlisting}[language=cpp]
// seperate the groups of nested parentheses

if (chr=='(')
{
    level+=1;
    current_paren+=chr;
}        
else if %*\wrongtok{chr==\textquotesingle{})\textquotesingle{}}*)
{
    %*\dots*)
    \end{lstlisting} &
    \begin{lstlisting}[language=cpp]
// seperate the groups of nested parentheses

if (chr=='(')
{
    level+=1;
    current_paren+=chr;
}        
else if %*\righttok{(chr==\textquotesingle{})\textquotesingle{})}*)
{
    %*\dots*)
    \end{lstlisting}
        \hspace{1pt}
        \\[5mm]
      
  \end{tabular}

\end{table}
\subsection{Case Study}
\label{sec:case-study}

% Define a custom color
\definecolor{mycrefcolor}{HTML}{0279AF} 

% Create a new command for coloring text
\newcommand{\colorcref}[1]{\textcolor{mycrefcolor}{#1}}

For a qualitative evaluation, we manually inspect instances where unconstrained decoding fails and our type constraining approach successfully corrects errors.
We showcase three such examples in \cref{fig:case-study}.

\paragraph{Preventing use of invalid types} In \cref{fig:case-study}\colorcref{a}, \dream{} generates a summary of a financial review for task \#30 in our \json{} dataset. The schema requires to output three key values as float numbers. Meanwhile, the model attempts generating the values as strings. Due to the derived language for the JSON schema, it can be determined that the strings are misplaced, not constituting one of the required keys and impossible to match the intended value formatting, and all attempts at placing such strings are thus rejected. Instead, the model generates the values without quote wrapping, resulting in a valid and correct result.

\paragraph{Preventing inadequate nesting}
In \cref{fig:case-study}\colorcref{b} \dreamcoder{} generates an invalid \smiles{} molecule for task \#166 by closing more parentheses than it opened. Since the CFG for SMILES correctly handles counting of nesting levels, attempts to generate the closing parenthesis are rejected by our method. Instead, the model decides to end the generation.

\paragraph{Preventing inadequate syntax}
In \cref{fig:case-study}\colorcref{c}, \deepseekcsevenb{} uses Python-style parentheses-less conditions in an if-statement when writing a string processing function in task \#150 of our \humaneval{} dataset. Since this is invalid in C++ syntax, our method can correct this mistake successfully, forcing the model to add parentheses around the condition.
